# Supplementary material for: Promising High Temperature Thermoelectric Performance of Alkali Metal-based Zintl phases X$_2$AgY (X = Na, K; Y = Sb, Bi): Insights from First-Principles Studies
Source: arXiv:2502.13680 source file (2025-02-19)
Supplement: Supplementary file 1 [file Supplemental.pdf]

# Supplementary: Promising High Temperature Thermoelectric Performance of Alkali Metal-based Zintl phases $X_2AgY$ ( $X = Na, K$ ; $Y = Sb, Bi$ ): Insights from First-Principles Studies

Mohd Zeeshan,<sup>1</sup> Indranil Mal,<sup>1</sup> and B. K. Mani<sup>1,\*</sup>

<sup>1</sup>*Department of Physics, Indian Institute of Technology, Hauz Khas, New Delhi 110016, India*

(Dated: February 19, 2025)

---

\* bkmani@physics.iitd.ac.in

## I. STRUCTURAL PARAMETERS (WYCKOFF POSITIONS)

$$\text{Na}_2\text{AgSb} = \begin{bmatrix} \text{Na} & 0.3217567218088941 & 0.3483320764351772 & 0.2500000000000000 \\ \text{Ag} & 0.5000000000000000 & 0.0000000000000000 & 0.0000000000000000 \\ \text{Sb} & 0.0000000000000000 & 0.2079399428763350 & 0.2500000000000000 \end{bmatrix}$$

$$\text{Na}_2\text{AgBi} = \begin{bmatrix} \text{Na} & 0.3194491394067498 & 0.3417801395542384 & 0.2500000000000000 \\ \text{Ag} & 0.5000000000000000 & 0.0000000000000000 & 0.0000000000000000 \\ \text{Bi} & 0.0000000000000000 & 0.1991791110046890 & 0.2500000000000000 \end{bmatrix}$$

$$\text{K}_2\text{AgSb} = \begin{bmatrix} \text{K} & 0.3275862389069361 & 0.3506477116588684 & 0.2499958619694425 \\ \text{Ag} & 0.4999911124200189 & 0.0000000000000000 & 0.0000000000000000 \\ \text{Sb} & 0.0000000000000000 & 0.2355668686592879 & 0.2500000000000000 \end{bmatrix}$$

$$\text{K}_2\text{AgBi} = \begin{bmatrix} \text{K} & 0.3262765125831701 & 0.3458200099664470 & 0.2500071714079896 \\ \text{Ag} & 0.5000014876499070 & 0.0000000000000000 & 0.0000000000000000 \\ \text{Bi} & 0.0000000000000000 & 0.2283611263530088 & 0.2500000000000000 \end{bmatrix}$$

## II. ELECTRONIC AND THERMAL PROPERTIES

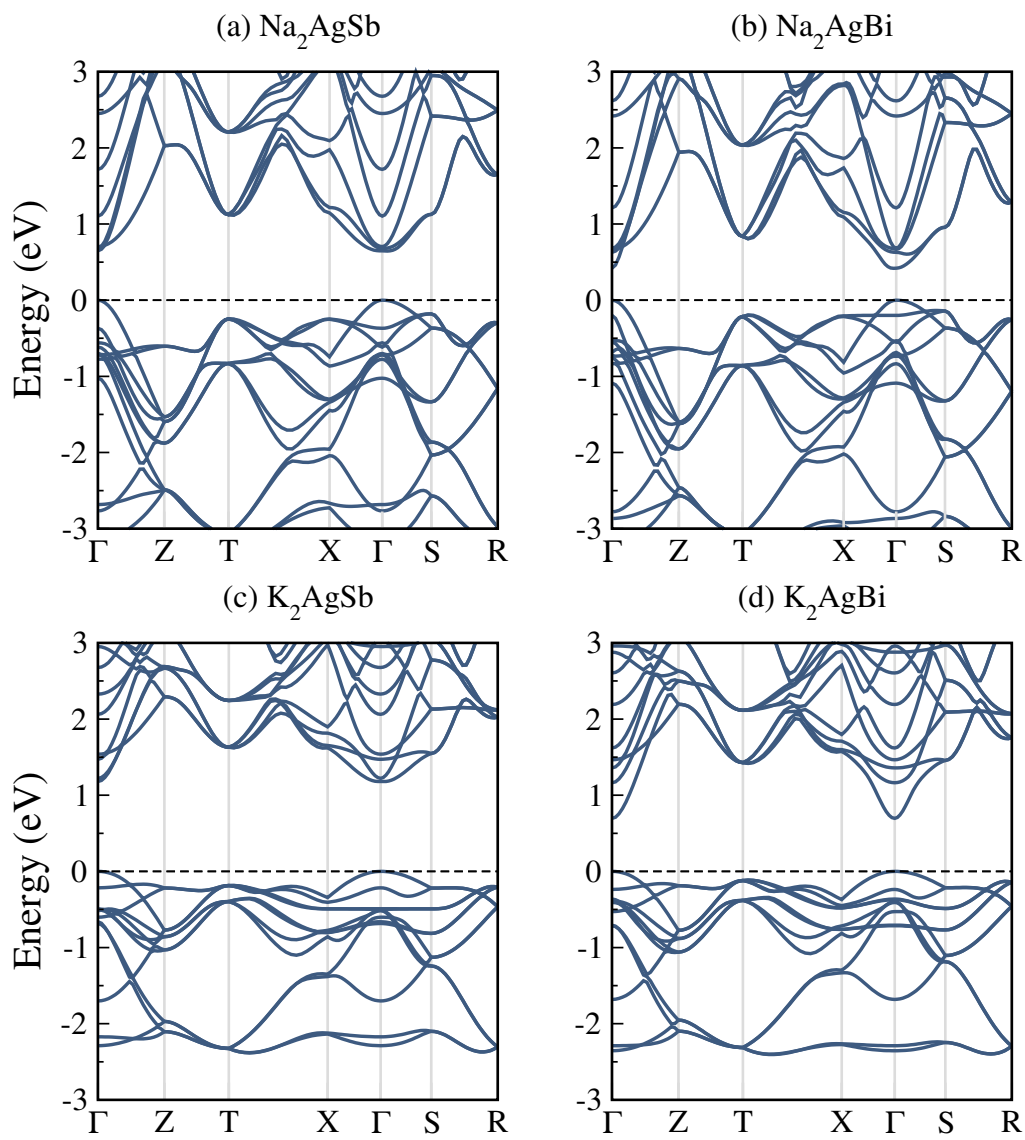

Figure S1: Calculated PBE electronic structures.

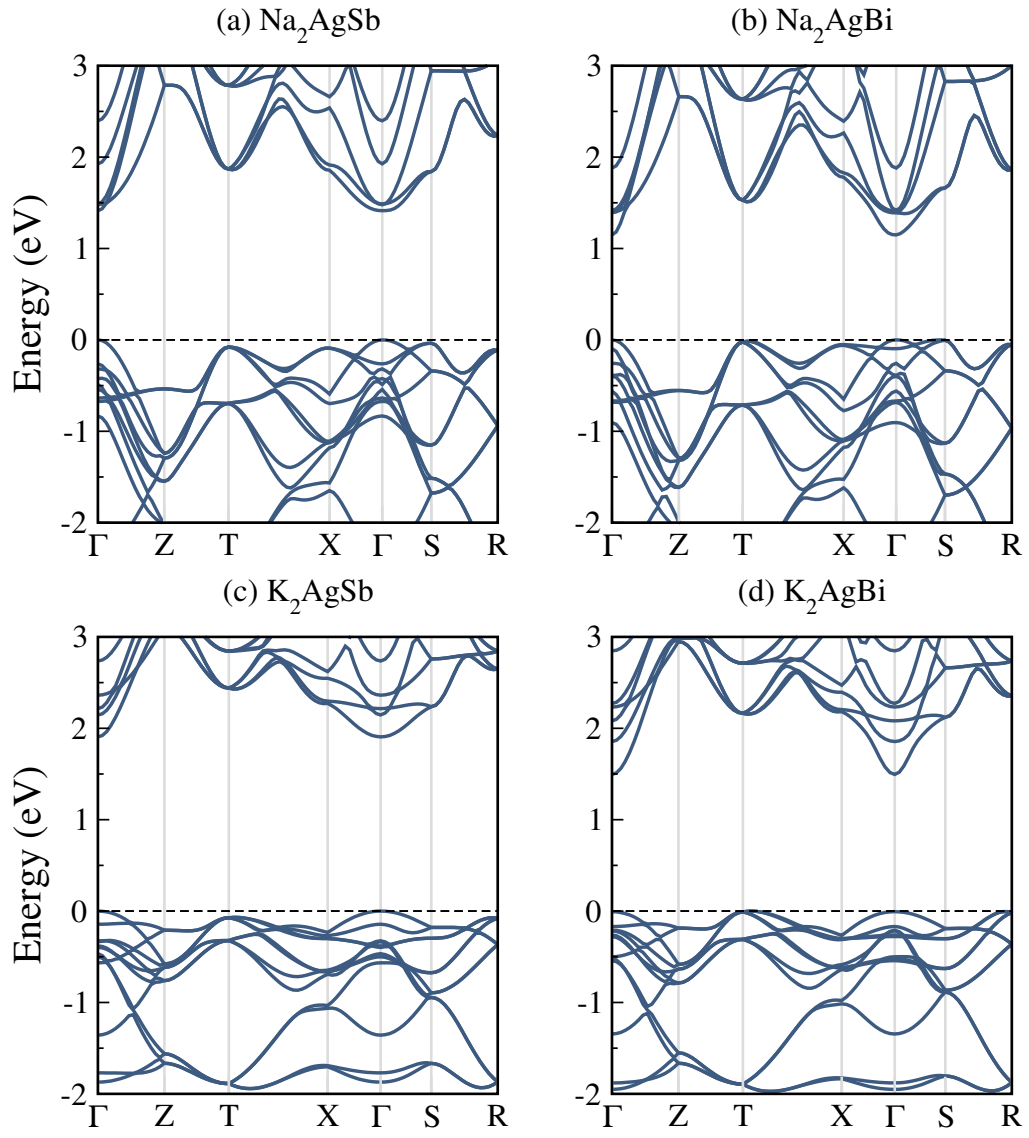

Figure S2: Calculated mBJ electronic structures.

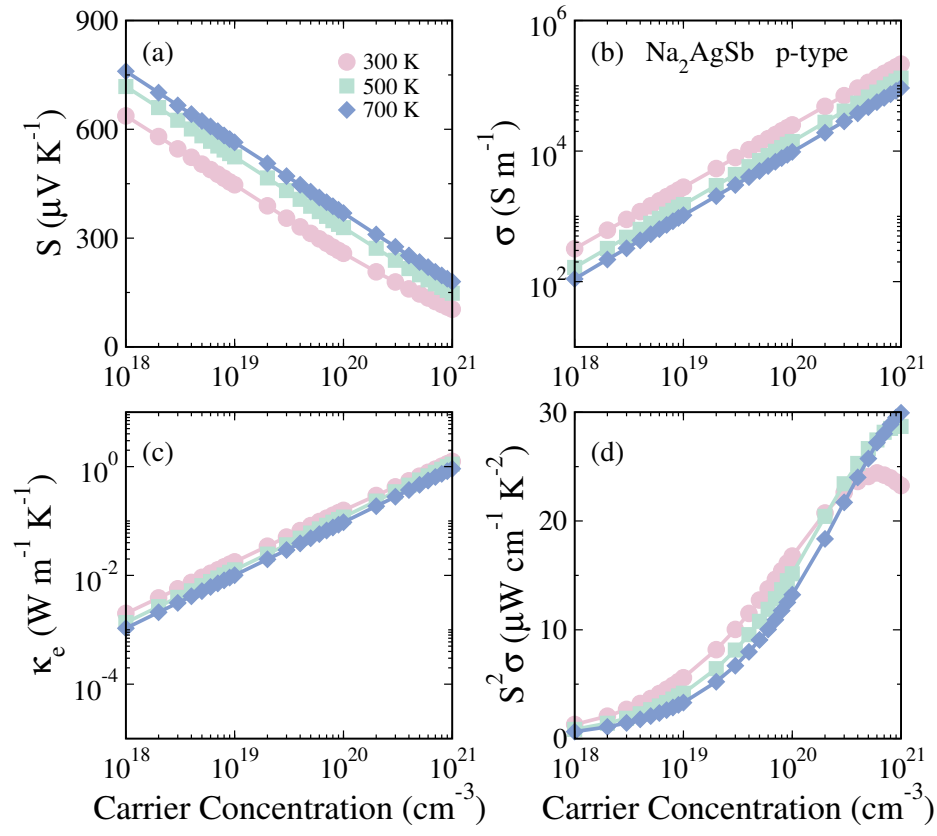

Figure S3: (a) Seebeck coefficient, (b) electrical conductivity, (c) electronic thermal conductivity, and (d) power factor for  $p$ -type  $\text{Na}_2\text{AgSb}$ .

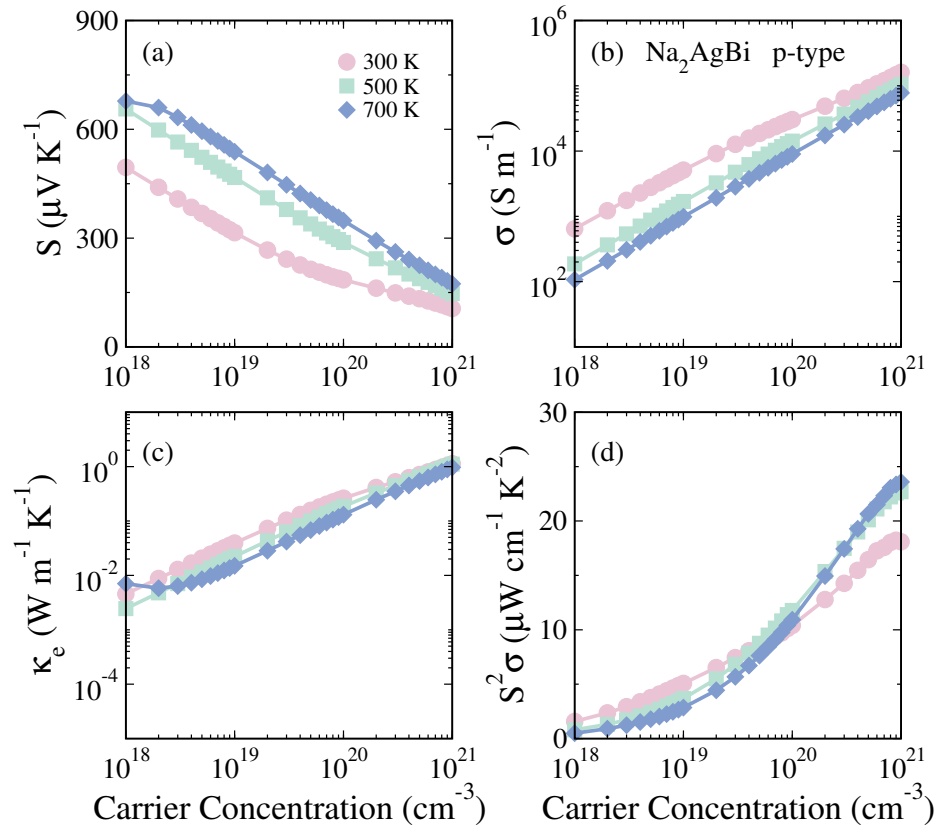

Figure S4: (a) Seebeck coefficient, (b) electrical conductivity, (c) electronic thermal conductivity, and (d) power factor for  $p$ -type  $\text{Na}_2\text{AgBi}$ .

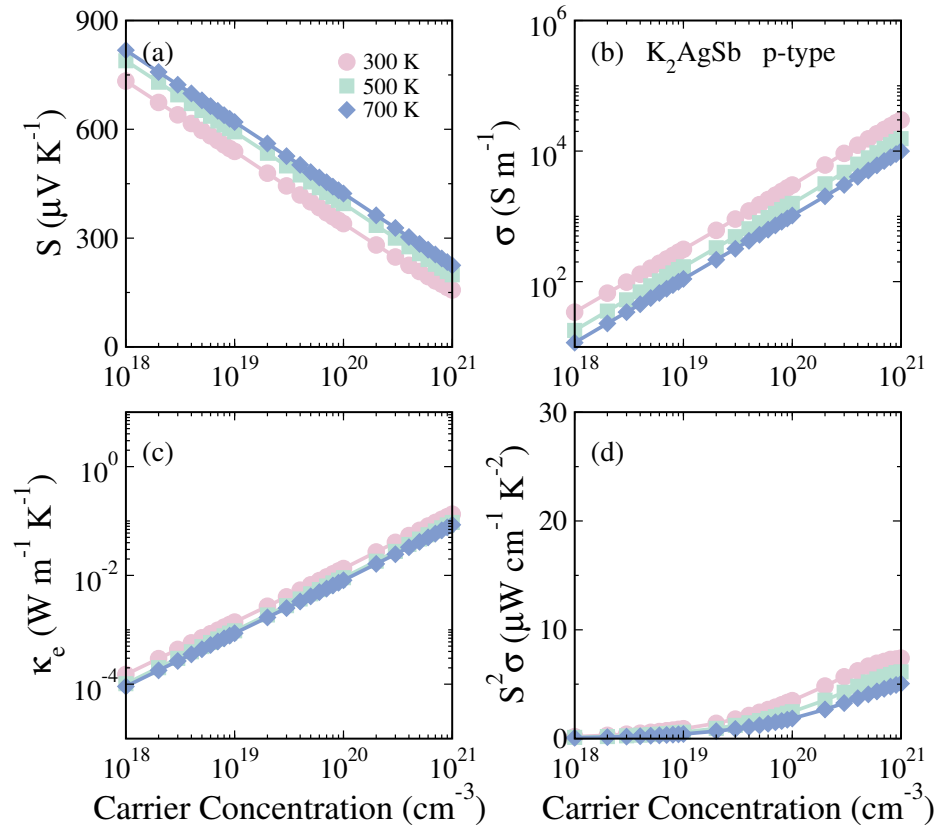

Figure S5: (a) Seebeck coefficient, (b) electrical conductivity, (c) electronic thermal conductivity, and (d) power factor for  $p$ -type  $\text{K}_2\text{AgSb}$ .

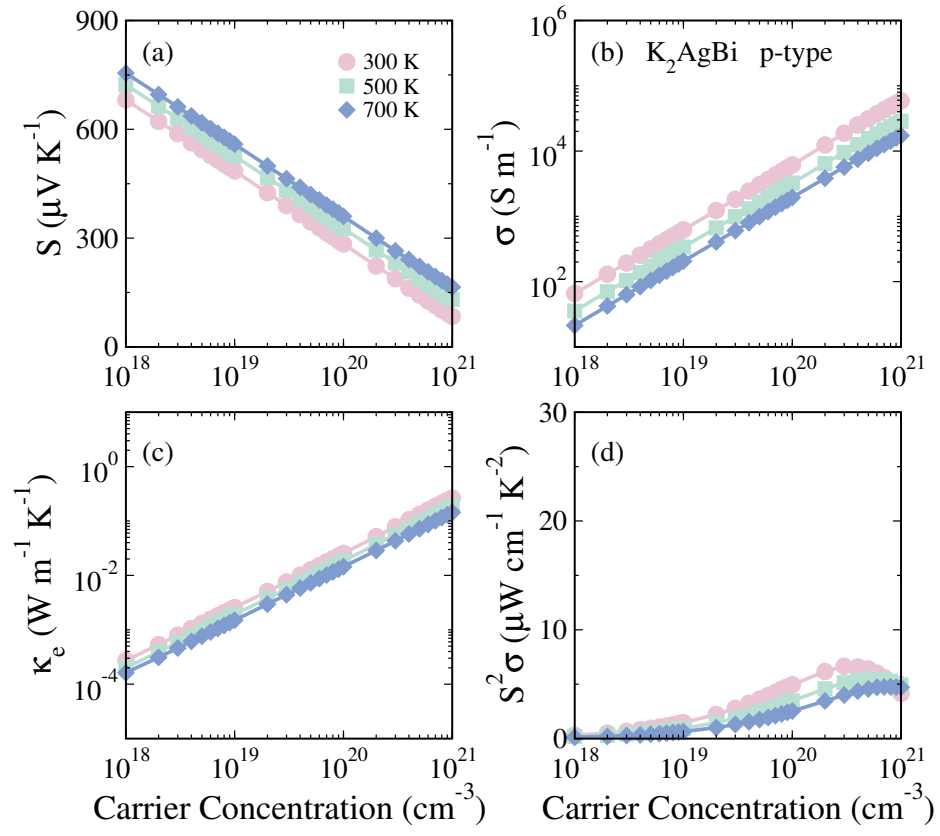

Figure S6: (a) Seebeck coefficient, (b) electrical conductivity, (c) electronic thermal conductivity, and (d) power factor for  $p$ -type  $\text{K}_2\text{AgBi}$ .



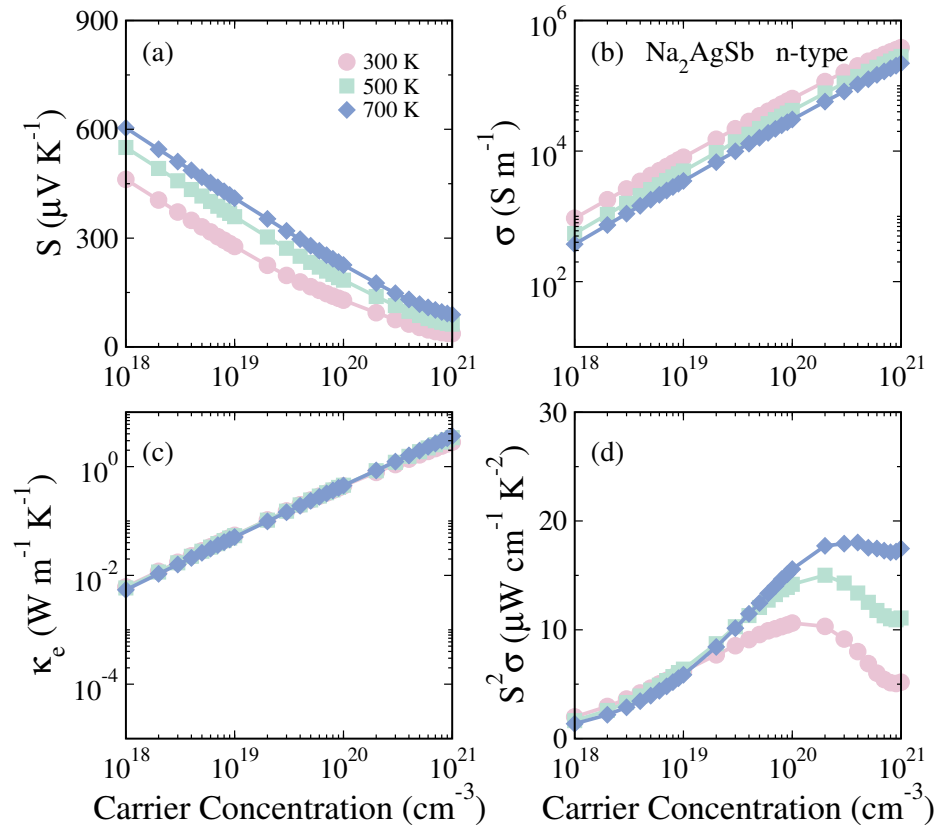

Figure S7: (a) Seebeck coefficient, (b) electrical conductivity, (c) electronic thermal conductivity, and (d) power factor for  $n$ -type  $\text{Na}_2\text{AgSb}$ .

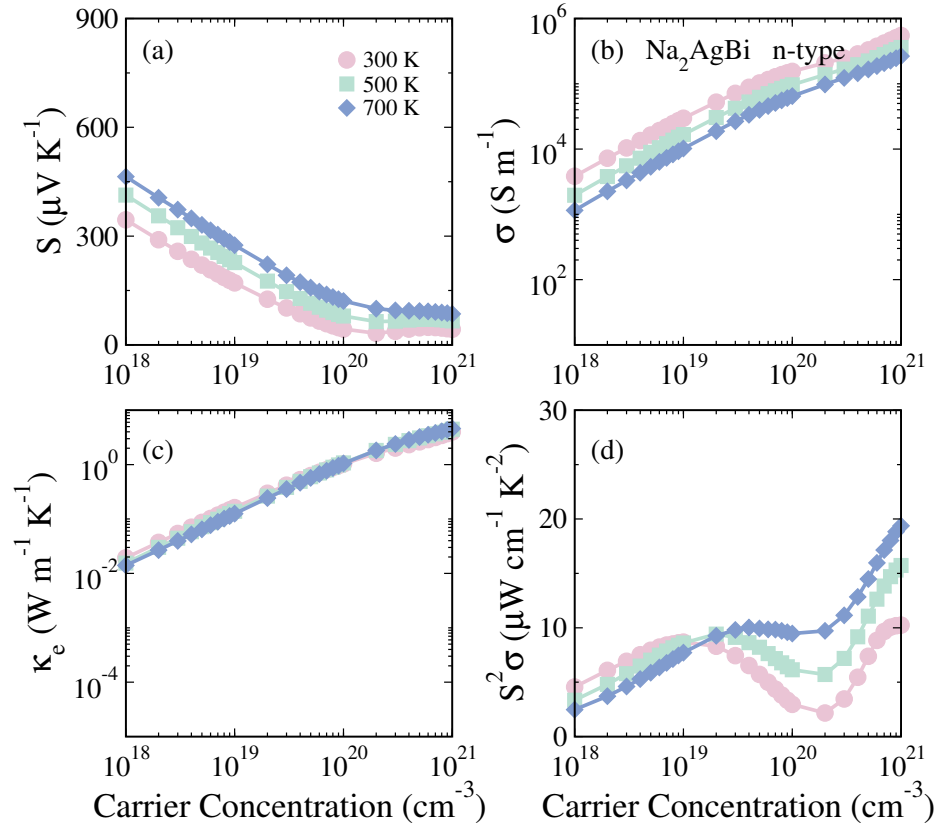

Figure S8: (a) Seebeck coefficient, (b) electrical conductivity, (c) electronic thermal conductivity, and (d) power factor for  $n$ -type  $\text{Na}_2\text{AgBi}$ .

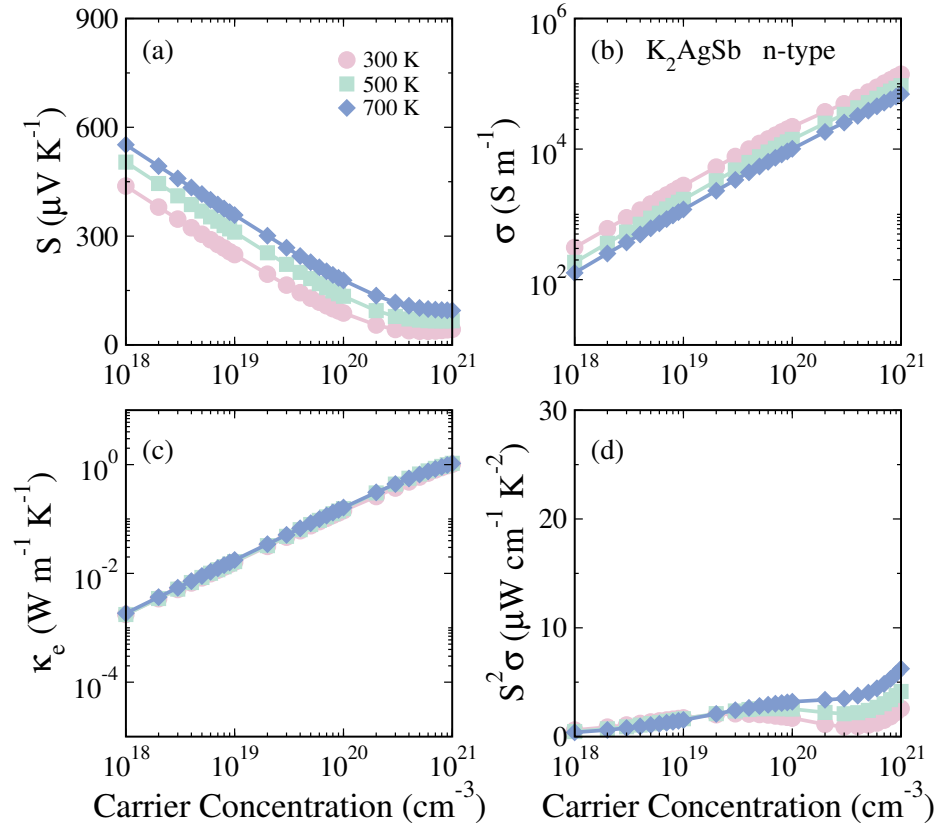

Figure S9: (a) Seebeck coefficient, (b) electrical conductivity, (c) electronic thermal conductivity, and (d) power factor for  $n$ -type  $\text{K}_2\text{AgSb}$ .

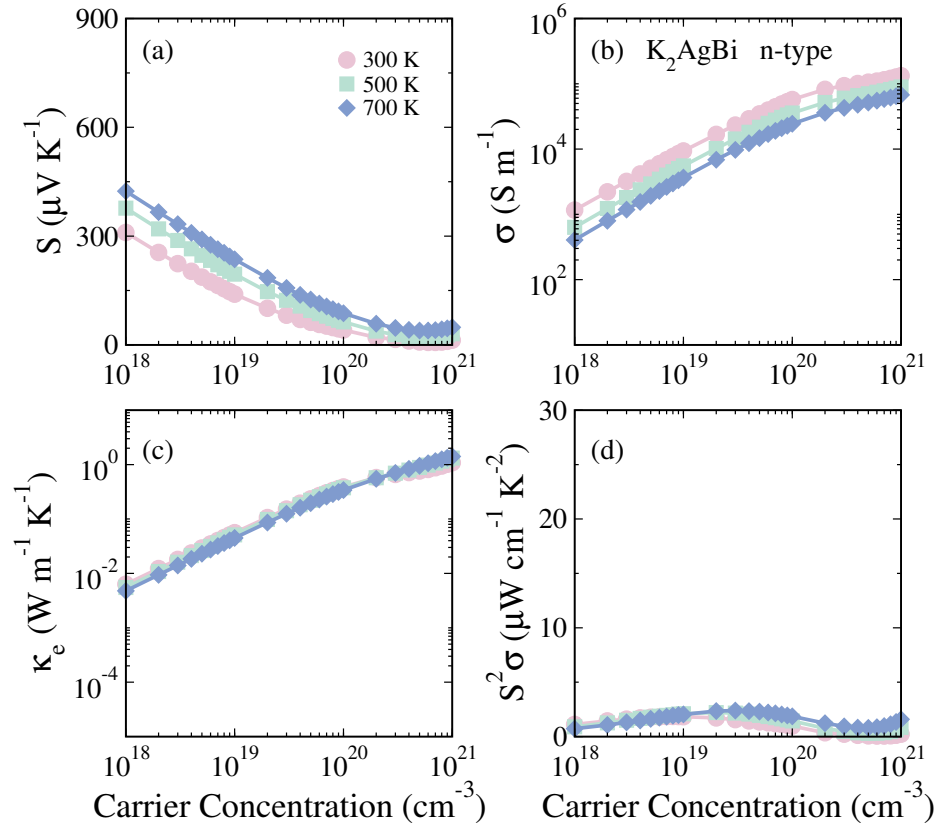

Figure S10: (a) Seebeck coefficient, (b) electrical conductivity, (c) electronic thermal conductivity, and (d) power factor for  $n$ -type  $\text{K}_2\text{AgBi}$ .

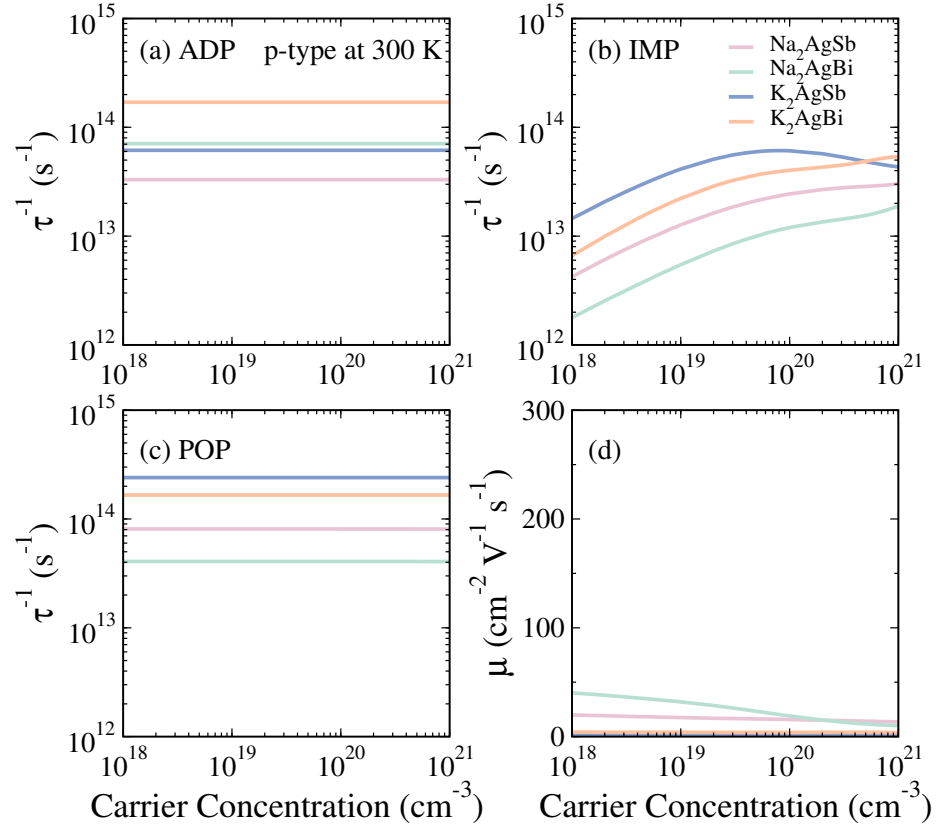

Figure S11: (a) ADP, (b) IMP, (c) POP scattering rates and (d) mobility for *p*-type  $\text{Na}_2\text{AgSb}$ ,  $\text{Na}_2\text{AgBi}$ ,  $\text{K}_2\text{AgSb}$ , and  $\text{K}_2\text{AgBi}$  at 300 K.

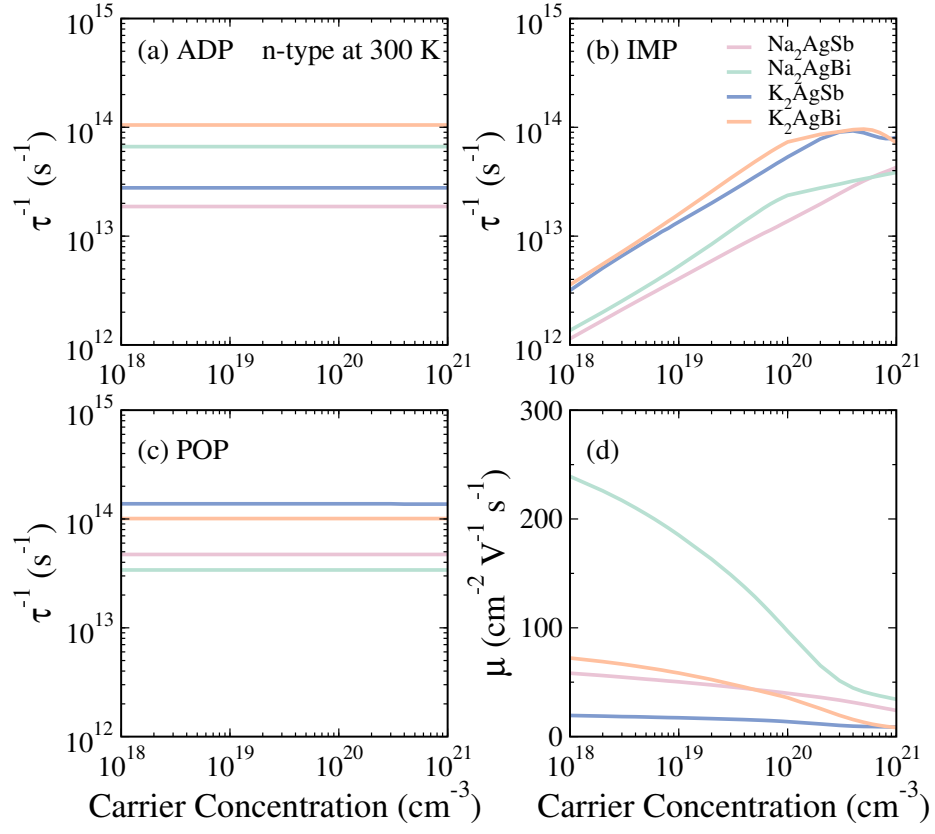

Figure S12: (a) ADP, (b) IMP, (c) POP scattering rates and (d) mobility for *n*-type Na<sub>2</sub>AgSb, Na<sub>2</sub>AgBi, K<sub>2</sub>AgSb, and K<sub>2</sub>AgBi at 300 K.

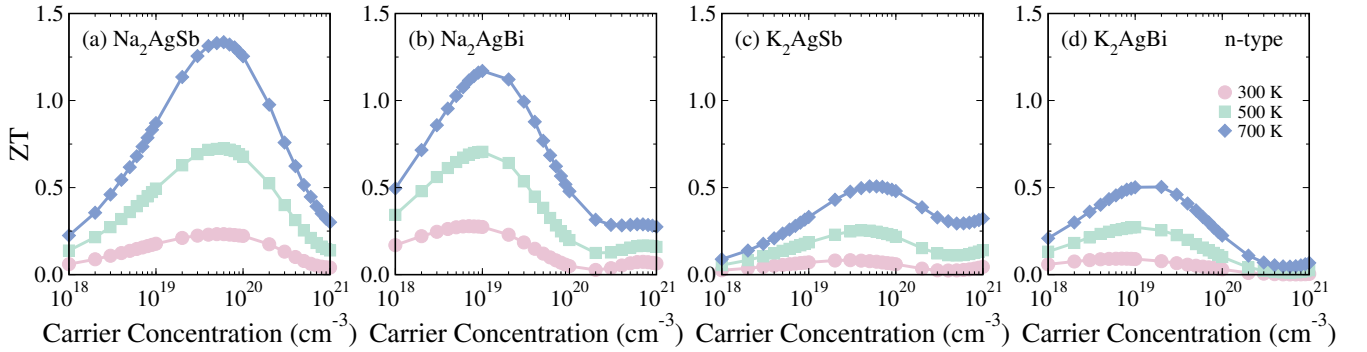

Figure S13: Figure of merit as a function of carrier concentration for *n*-type (a) Na<sub>2</sub>AgSb, (b) Na<sub>2</sub>AgBi, (c) K<sub>2</sub>AgSb, and (d) K<sub>2</sub>AgBi.

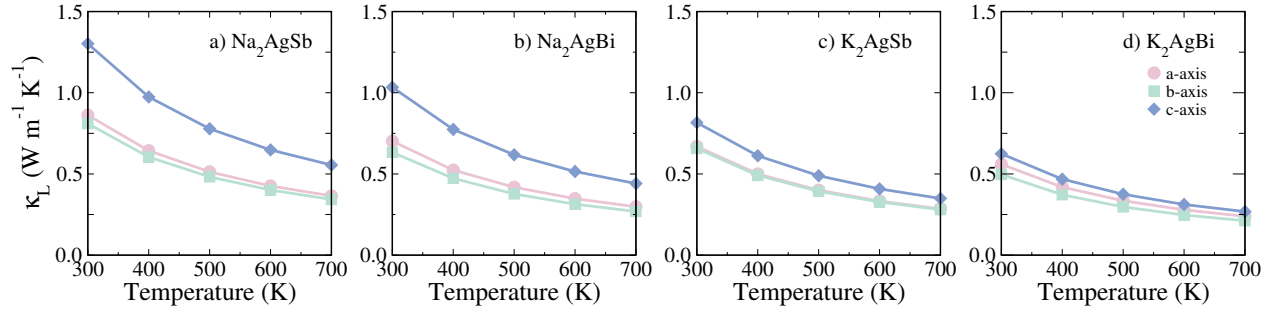

Figure S14: Lattice thermal conductivity of (a)  $\text{Na}_2\text{AgSb}$ , (b)  $\text{Na}_2\text{AgBi}$ , (c)  $\text{K}_2\text{AgSb}$ , and (d)  $\text{K}_2\text{AgBi}$ , along different crystallographic directions.

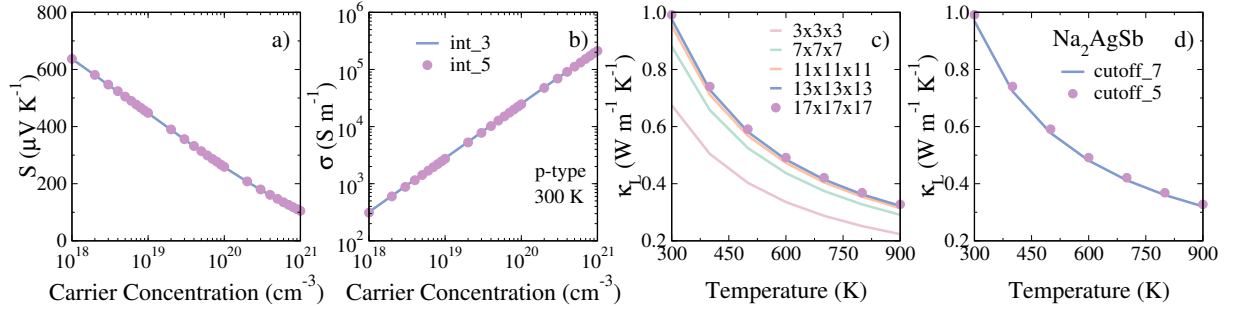

Figure S15: Convergence test of (a) Seebeck coefficient, (b) electrical conductivity, and [(c), (d)] lattice thermal conductivity. The values in filled circles are used in the manuscript.
